# Supplementary material for: Interpretable models for extrapolation in scientific machine learning
Source: arXiv:2212.10283 source file (2022-12-16)
Supplement: Supplementary file 1 [file Muckley_et_al_Supporting_Info.pdf]

# SUPPORTING INFORMATION
## Interpretable models for extrapolation in scientific machine learning

Eric S. Muckley[1], James E. Saal[1], Bryce Meredig[1], Christopher S. Roper[2], John H. Martin[2]

[1]Citrine Informatics, Redwood City, 94063, CA, USA
[2]HRL Laboratories, Malibu, 90265, CA, USA

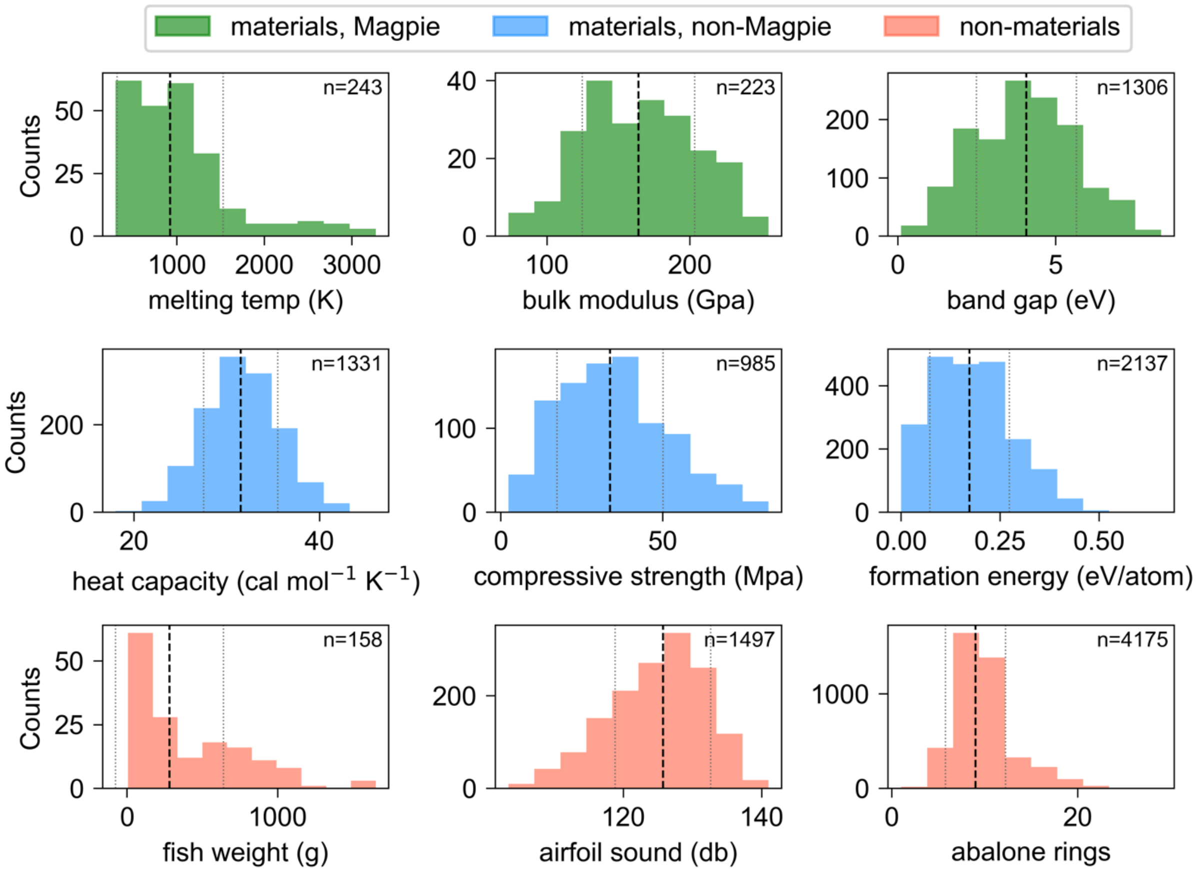


Figure S1. Histograms of the target variable distribution of each test dataset, which include materials datasets featurized using Magpie (top row, green), materials datasets without Magpie features (middle row, blue), and non-materials datasets (bottom row, red). Vertical dashed lines show the median target value of each dataset along with its standard deviation.

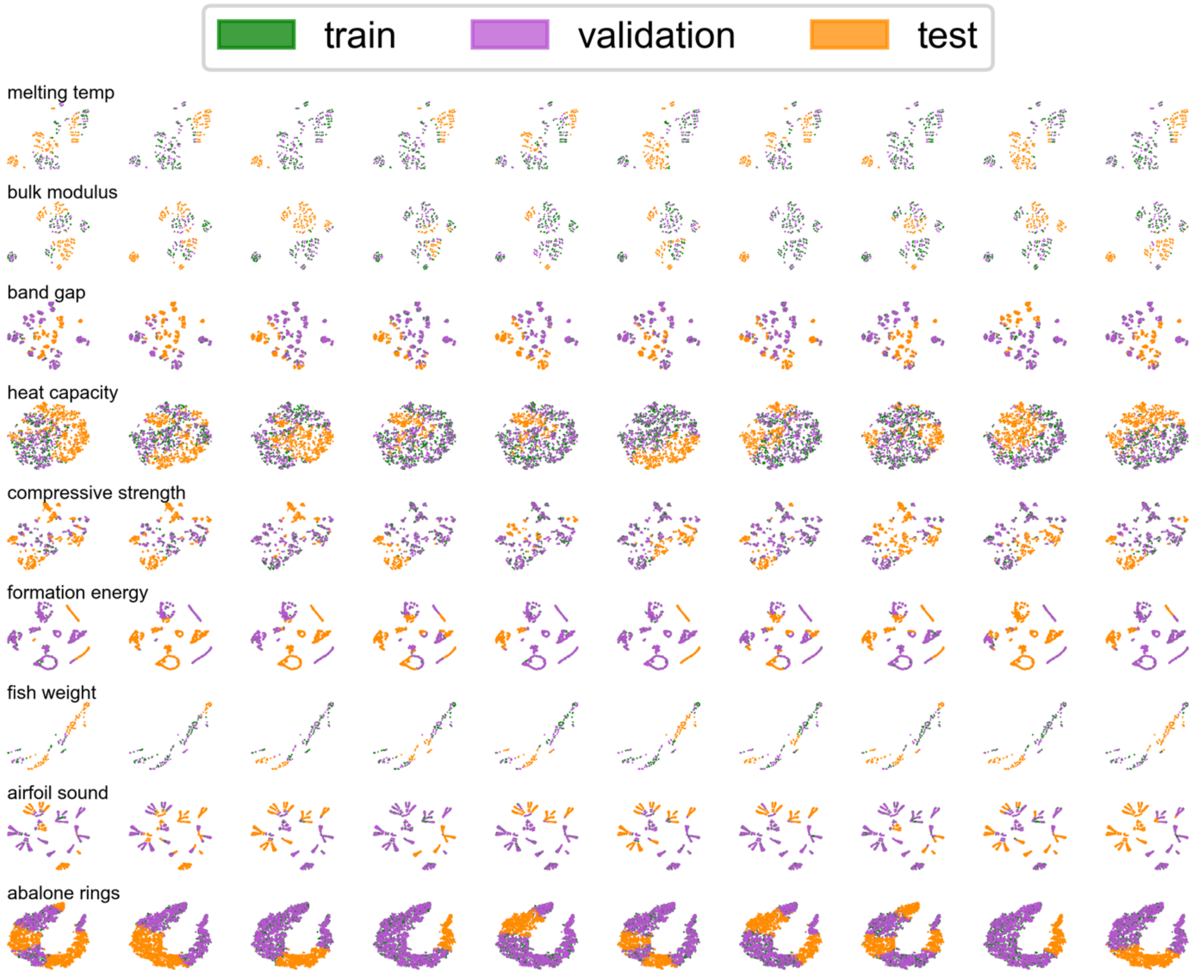


Figure S2. Visualization of datasets in 2-dimensional t-SNE[1] space (each row corresponds to 1 dataset) showing example partitions used for LOCO CV to test model extrapolation (each column corresponds to 1 CV split). At each CV split, train (green) points were used for training regression models, validation (purple) points were used for feature engineering, and test (orange) points were used for evaluating model performance.

[1] Van der Maaten, L. and Hinton, G., 2008. Visualizing data using t-SNE. *Journal of machine learning research*, *9*(11).

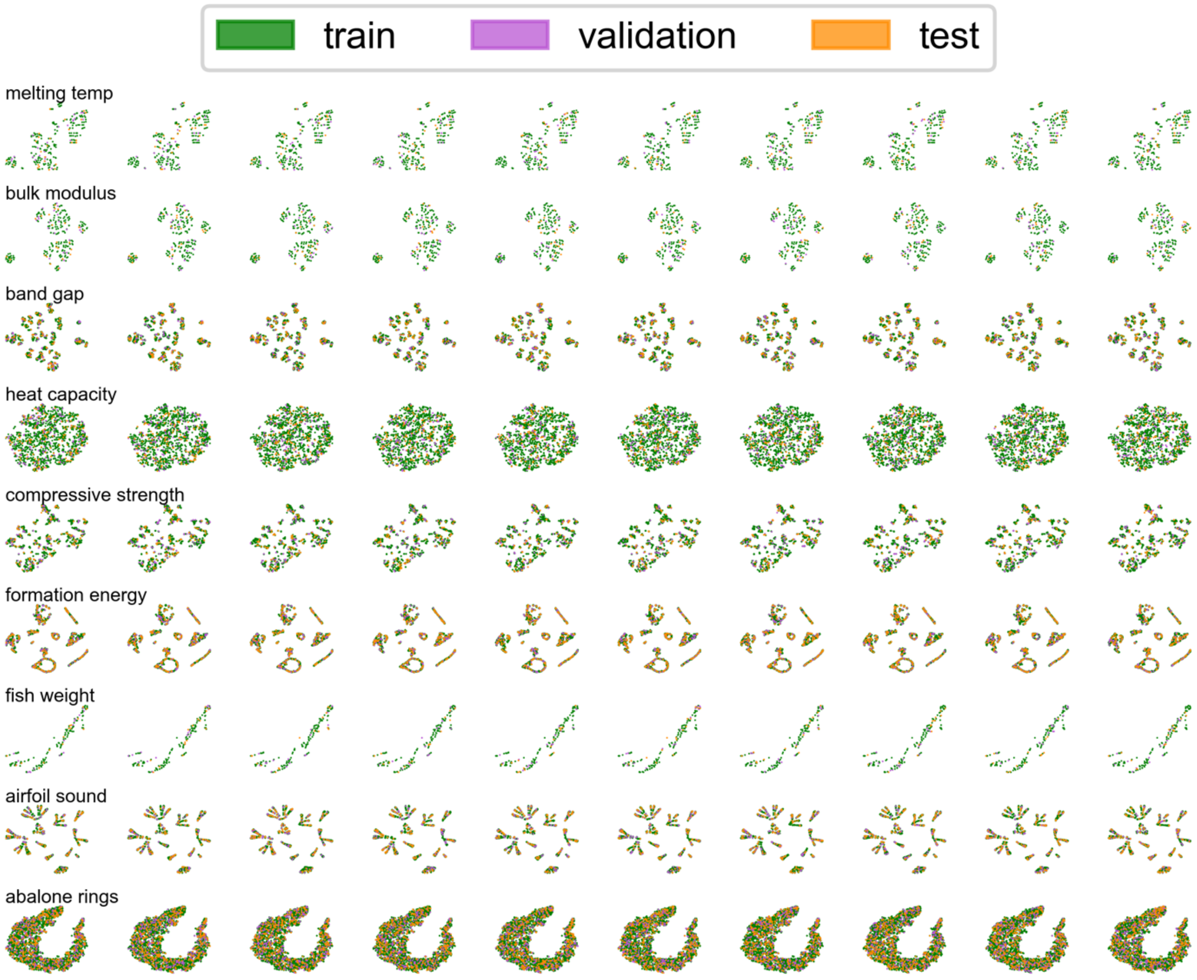


Figure S3. Visualization of datasets in 2-dimensional t-SNE space (each row corresponds to 1 dataset) showing example partitions used for random CV to test model interpolation (each column corresponds to 1 CV split). At each CV split, train (green) points were used for training regression models, validation (purple) points were used for feature engineering, and test (orange) points were used for evaluating model performance.

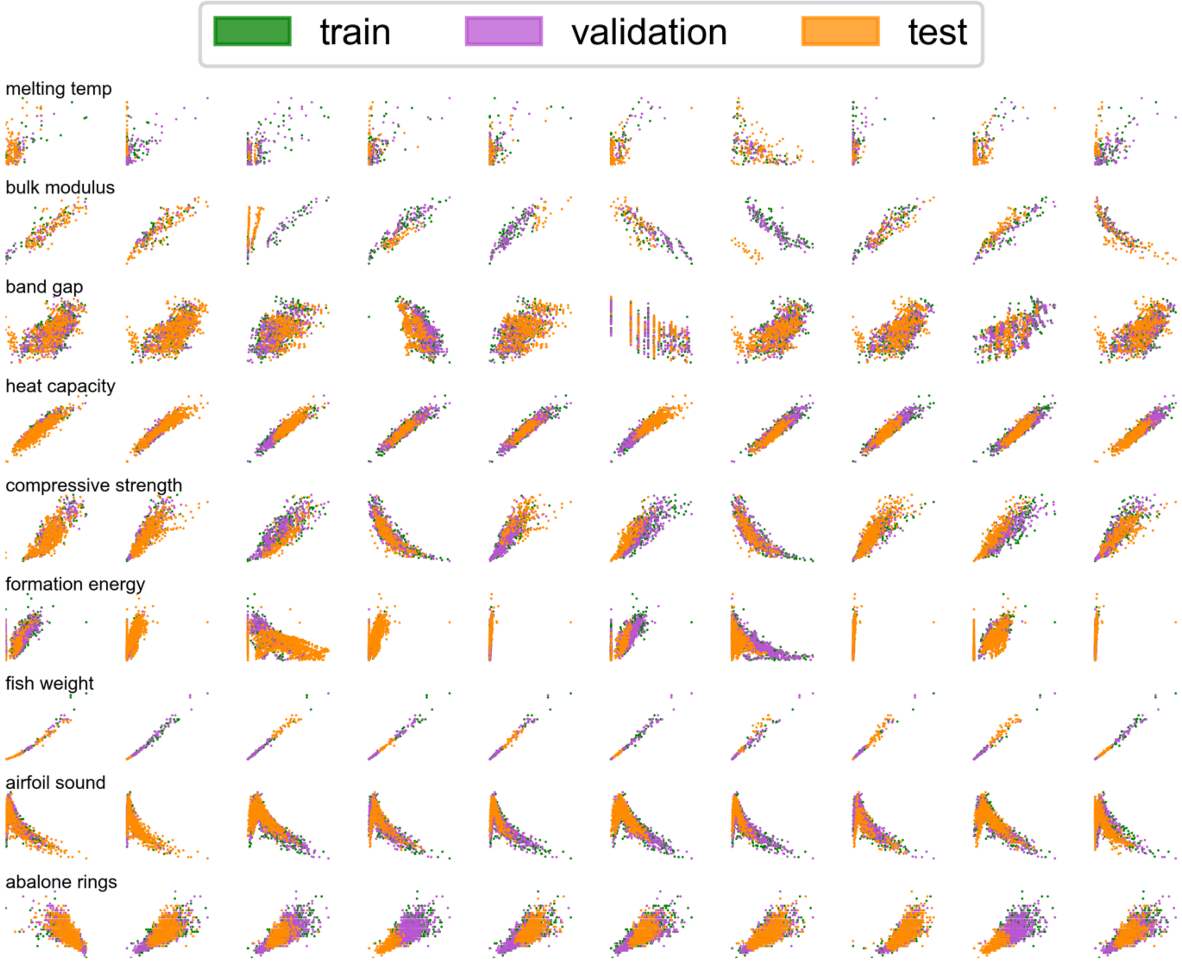


Figure S4. Visualization of the best feature found at each CV split for extrapolation. Each row corresponds to a single dataset, and each column corresponds to a single LOCO CV split. Each panel represents the values of the target variable (vertical axis) plotted against the values of the best engineered feature found at that CV split. Engineered features were selected only on their correlation to the target values in the validation set (purple), while the train (green) and test (orange) points were used for training and testing of regression models.

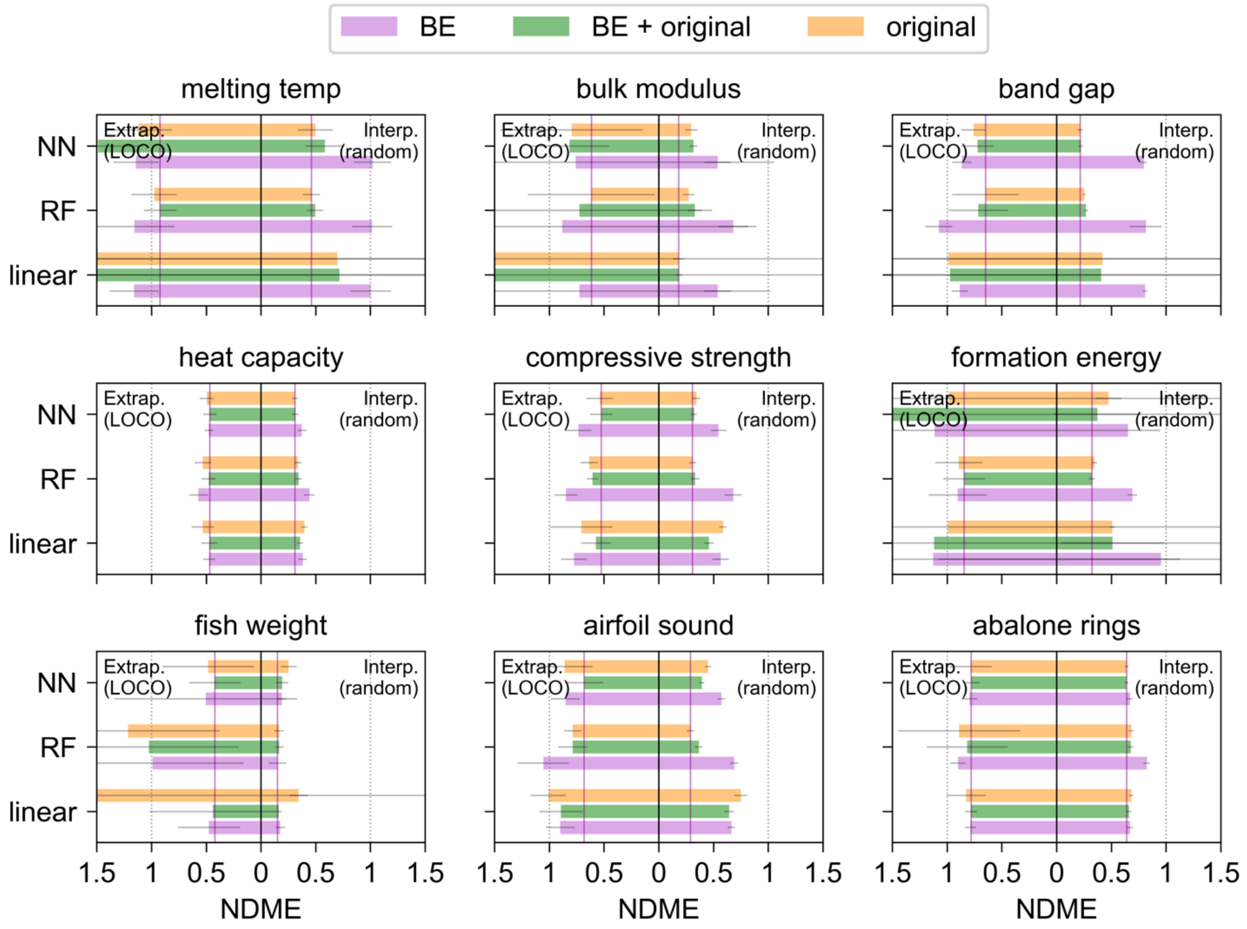


Figure S5. Comparison of model extrapolation and interpolation performance, as quantified by median NDME for 3 different regression types (linear, random forest, and neural network, on the vertical axis), and 3 different featurization strategies: (1) original: the model was trained using only the original input features in the dataset, including those calculated using Magpie, (2) best engineered (BE): the model was trained using the single best engineered input feature for the given CV split as ranked by its $r^2$ correlation to the validation set, and (3) BE + original: the model was trained using all original input features and the single best engineered feature. Each panel corresponds to a single dataset, where the left-hand side of the panel shows median NDME for LOCO CV (extrapolation) and the right-hand side of the panel shows median NDME for random CV (interpolation). Error bars correspond to standard deviation in NDME across all train-test splits for a given model configuration. Solid vertical lines correspond to the lowest model error recorded for a given extrapolation/interpolation task.
